# Supplementary material for: The Hellan-Herrmann-Johnson method with curved elements
Source: arXiv:1909.09687 ancillary file (2020-07-25)
Supplement: Supplementary file 1 [file Curved_HHJ_supplement.pdf]

# SUPPLEMENTARY MATERIALS: THE HELLAN–HERRMANN–JOHNSON METHOD WITH CURVED ELEMENTS*

DOUGLAS N. ARNOLD† AND SHAWN W. WALKER‡

For the convenience of the reader, we collect several basic results that are useful to the main paper.

**SM1. Proof of Proposition 2.1.** Using (2.8), we may estimate the skeleton term in (2.12) by

$$\begin{aligned} h\|v\|^2_{L^2(\mathcal{E}_h)} &\leq \sum_{T\in\mathcal{T}_h} h\|v\|^2_{L^2(\partial T)} \leq C_3 \sum_{T\in\mathcal{T}_h} \|v\|^2_{L^2(T)} + h^2\|\nabla v\|^2_{L^2(T)} \\ &\leq C_3\left(\|v\|^2_{L^2(\Omega)} + h^2\|\nabla v\|^2_{L^2(\Omega)}\right), \end{aligned} \tag{SM1.1}$$

which gives the result.

**SM2. Background of Curved Finite Elements.** We review the theory in [SM5].

**SM2.1. Parametric Elements.** Let $\mathcal{P}_l(\mathcal{D}) \equiv \mathcal{P}_l(\mathcal{D};\mathbb{R})$ be the space of polynomials of degree $\leq l$ on the generic domain $\mathcal{D}$ (for $l \geq 0$), and let $\widehat{T}$ be the reference unit triangle. We introduce the set of Lagrange nodal variables (points) $\mathcal{N}_l(\widehat{T}) \equiv \widehat{\mathcal{N}}_l$ on $\widehat{T}$ that correspond to $\mathcal{P}_l(\widehat{T}) \equiv \widehat{\mathcal{P}}_l$, with associated (point evaluation) Lagrange interpolation operator $\hat{\dot{\mathcal{I}}}_l$. Thus, the reference finite element is the triple $(\widehat{T}, \widehat{\mathcal{N}}_l, \widehat{\mathcal{P}}_l)$.

Let $\boldsymbol{A}_T : \widehat{T} \to T^1$ be an affine map that generates a straight triangle $T^1 \in \mathcal{T}_h^1$, with polynomial space $\mathcal{P}_l^1 \equiv \mathcal{P}_l^1(T^1)$, corresponding finite element triple $(T^1, \mathcal{N}_l^1, \mathcal{P}_l^1)$, and Lagrange interpolation operator $\dot{\mathcal{I}}_l^1$. Let $T^m = \boldsymbol{F}_T^m(T^1)$ be a curved triangle, where $[\mathcal{P}_m(\widehat{T})]^2 \ni \boldsymbol{F}_T^m : T^1 \to T^m$ is a regular invertible mapping (and $m \geq 1$). This induces a mapped polynomial space

$$\mathcal{P}_l^m \equiv \mathcal{P}_l^m(T^m) = \{\hat{p} \circ (\boldsymbol{F}_T^m)^{-1} \mid \hat{p} \in \mathcal{P}_l^1\}, \tag{SM2.1}$$

with mapped nodal set given by $\mathcal{N}_l^m \equiv \mathcal{N}_l^m(T^m) = \{\boldsymbol{F}_T^m(\mathbf{a}) \mid \mathbf{a} \in \mathcal{N}_l^1\}$. Hence, the "parametric" finite element is the triple $(T^m, \mathcal{N}_l^m, \mathcal{P}_l^m)$, with Lagrange interpolation operator given by $\dot{\mathcal{I}}_l^m(f) \circ \boldsymbol{F}_T^m = \dot{\mathcal{I}}_l^1(f \circ \boldsymbol{F}_T^m)$.

In general, there is no relation between $l$ and $m$. Typically, $l = m$ refers to the *iso-parametric* case. We use the notation $\boldsymbol{F}_T^\infty \equiv \boldsymbol{F}_T$ to indicate a general non-linear map (not necessarily a polynomial) that maps $T^1$ to a triangle $T \in \mathcal{T}_h$, and the same considerations above apply to this case as well.

Note that $m = 1$ indicates linear (straight) triangles and there are well-known procedures for generating a conforming, shape regular triangulation, consisting of linear triangles, that approximates a smooth domain. Generating higher order triangles,

---

*Submitted to the editors DATE.
**Funding:** This article is based upon work supported by the National Science Foundation under grants DMS-1719694 (Arnold) and DMS-155222 (Walker) and by the Simons Foundations under grant 601937 (Arnold).
†Department of Mathematics, University of Minnesota, Minneapolis (arnold@umn.edu, http://umn.edu/~arnold/).
‡Department of Mathematics, Louisiana State University, Baton Rouge (walker@lsu.edu, http://www.math.lsu.edu/~walker/).

$T^m$, that approximate the domain better than linears, requires an "optimal" map $\boldsymbol{F}_T^m$ which is defined by the procedure in [SM5]. The next section highlights the properties of these maps.

**SM2.2. Approximation of $\Omega$ by $\Omega^m$.** The following results [SM5, Lemma 5, Propositions 2, 3] give estimates on how well $\Omega^m$ approximates $\Omega$. Let $\boldsymbol{\Psi}_T^m : T^m \to T$, for each $T \in \mathcal{T}_h$, and note that $\boldsymbol{\Psi}_T^1 \equiv \boldsymbol{F}_T$.

PROPOSITION SM2.1 (Forward Map). *Let $1 \le m \le k$. The map $\boldsymbol{\Psi}_T^m$ satisfies the following properties:*

1. *There exist constants $b_s > 0$, independent of $h$, such that*

$$\|\nabla^s((\boldsymbol{\Psi}_T^m - \mathrm{id}_{T^m}) \circ \boldsymbol{F}_T^m \circ \boldsymbol{A}_T)\|_{L^\infty(\widehat{T})} \le b_s h^{m+1}, \ \forall\ s \le m+1. \tag{SM2.2}$$

2. *There exist constants $\gamma_s > 0$, independent of $h$, such that*

$$\|\nabla^s(\boldsymbol{\Psi}_T^m - \mathrm{id}_{T^m})\|_{L^\infty(T^m)} \le \gamma_s h^{m+1-s}, \ \forall\ s \le m+1. \tag{SM2.3}$$

3. *$\boldsymbol{\Psi}_T^m$ is a $C^{m+1}$ diffeomorphism: $T^m \to T$.*
4. *There exists $\gamma > 0$, independent of $h$, such that*

$$\|\det(\nabla \boldsymbol{\Psi}_T^m) - 1\|_{L^\infty(T^m)} \le \gamma h^m. \tag{SM2.4}$$

PROPOSITION SM2.2 (Inverse Map). *Let $1 \le m \le k$. The inverse map $(\boldsymbol{\Psi}_T^m)^{-1} : T \to T^m$ satisfies the following properties:*

1. *There exist constants $\rho_s > 0$, independent of $h$, such that*

$$\|\nabla^s((\boldsymbol{\Psi}_T^m)^{-1} - \mathrm{id}_T)\|_{L^\infty(T)} \le \rho_s h^{m+1-s}, \ \forall\ s \le m+1. \tag{SM2.5}$$

2. *There exists $\rho > 0$, independent of $h$, such that*

$$\|\det(\nabla(\boldsymbol{\Psi}_T^m)^{-1}) - 1\|_{L^\infty(T)} \le \rho h^m. \tag{SM2.6}$$

**SM2.3. Proof of Theorem 3.2.** We break the result up into Theorem SM2.3, Corollary SM2.4, and Corollary SM2.5.

THEOREM SM2.3. *The map $\boldsymbol{\Phi}_T^{lm} = \boldsymbol{F}_T^m \circ (\boldsymbol{F}_T^l)^{-1}$, given in (3.1), satisfies a variant of (SM2.3) and (SM2.5), i.e.*

$$\begin{aligned} \|\nabla^s(\boldsymbol{\Phi}_T^{lm} - \mathrm{id}_{T^l})\|_{L^\infty(T^l)} &\le C h^{l+1-s}, \\ \|\nabla^s((\boldsymbol{\Phi}_T^{lm})^{-1} - \mathrm{id}_{T^m})\|_{L^\infty(T^m)} &\le C h^{l+1-s}, \end{aligned} \tag{SM2.7}$$

*for $0 \le s \le l+1$, where $C$ only depends on $\Gamma$.*

*Proof.* By the triangle inequality and (SM2.3),

$$\begin{aligned} \|\nabla^s(\boldsymbol{\Phi}_T^{lm} - \mathrm{id}_{T^l})\|_{L^\infty(T^l)} &\le \|\nabla^s(\boldsymbol{\Phi}_T^{lm} - \boldsymbol{\Psi}_T^l)\|_{L^\infty(T^l)} + \|\nabla^s(\boldsymbol{\Psi}_T^l - \mathrm{id}_{T^l})\|_{L^\infty(T^l)} \\ &\le \|\nabla^s\left[(\boldsymbol{\Psi}_T^l \circ (\boldsymbol{\Phi}_T^{lm})^{-1} - \mathrm{id}_{T^m}) \circ \boldsymbol{\Phi}_T^{lm}\right]\|_{L^\infty(T^l)} + C h^{l+1-s} \\ &\le \|\nabla^s\left[(\boldsymbol{\Psi}_T^m - \mathrm{id}_{T^m}) \circ \boldsymbol{\Phi}_T^{lm}\right]\|_{L^\infty(T^l)} + C h^{l+1-s}, \end{aligned} \tag{SM2.8}$$

where we used that $\boldsymbol{\Psi}_T^l \circ (\boldsymbol{\Phi}_T^{lm})^{-1} = \boldsymbol{F}_T \circ (\boldsymbol{F}_T^l)^{-1} \circ \boldsymbol{F}_T^l \circ (\boldsymbol{F}_T^m)^{-1} = \boldsymbol{F}_T \circ (\boldsymbol{F}_T^m)^{-1} = \boldsymbol{\Psi}_T^m$. Next, let $\widetilde{\boldsymbol{F}_T^l} := \boldsymbol{F}_T^l \circ \boldsymbol{A}_T : \widehat{T} \to T^l$ (for all $l \le m$) and note that

$$\|\nabla \boldsymbol{F}_T^l\|_{L^\infty(T^1)} \le \|\nabla \widetilde{\boldsymbol{F}_T^l}\|_{L^\infty(\widehat{T})} \|(\nabla \boldsymbol{A}_T)^{-1}\|_{L^\infty(\widehat{T})} \le C_1 h C_2 h^{-1} \le C', \tag{SM2.9}$$

where we used [SM5, Thm. 1] on $\nabla\widetilde{\boldsymbol{F}_T^l}$ (because $\boldsymbol{F}_T^l$ is an optimal map), $\boldsymbol{A}_T$ is the standard affine map, and $C' > 0$ is a uniform constant only depending on $\Gamma$. From this, we get

$$\begin{aligned} \nabla\boldsymbol{\Phi}_T^{lm} &= \nabla[\boldsymbol{F}_T^m \circ (\boldsymbol{F}_T^l)^{-1}] = [(\nabla\boldsymbol{F}_T^m)(\nabla\boldsymbol{F}_T^l)^{-1}] \circ (\boldsymbol{F}_T^l)^{-1}, \\ \Rightarrow \quad \|\nabla\boldsymbol{\Phi}_T^{lm}\|_{L^\infty(T^l)} &\le C\|\nabla\boldsymbol{F}_T^m\|_{L^\infty(T^1)}\|(\nabla\boldsymbol{F}_T^l)^{-1}\|_{L^\infty(T^1)} \le C'. \end{aligned} \tag{SM2.10}$$

Therefore,

$$\begin{aligned} &\|\nabla^s\left[(\boldsymbol{\Psi}_T^m - \mathrm{id}_{T^m}) \circ \boldsymbol{\Phi}_T^{lm}\right]\|_{L^\infty(T^l)} \\ &\quad \le C\sum_{j=1}^{s}\|\nabla^j(\boldsymbol{\Psi}_T^m - \mathrm{id}_{T^m})\|_{L^\infty(T^m)}\|\nabla^{s-j+1}\boldsymbol{\Phi}_T^{lm}\|_{L^\infty(T^l)} \le Ch^{l+1-s}, \end{aligned} \tag{SM2.11}$$

for $0 \le s \le l+1$, where we used the product rule, (SM2.3), (SM2.10), and many inverse estimates. Combining with (SM2.8) gives the first estimate in (SM2.7); the other estimate follws similarly. ∎

Corollary SM2.4. *The maps* $\boldsymbol{F}_T^m$, $\boldsymbol{F}_T^l$ *satisfy*

$$\begin{aligned} \|\nabla^s(\boldsymbol{F}_T^l - \mathrm{id}_{T^1})\|_{L^\infty(T^1)} &\le Ch^{2-s}, \quad \text{for} \ \ s = 0,1,2, \\ \|\nabla^s(\boldsymbol{F}_T^m - \boldsymbol{F}_T^l)\|_{L^\infty(T^1)} &\le Ch^{l+1-s}, \quad \text{for} \ \ 0 \le s \le l+1, \end{aligned} \tag{SM2.12}$$

*and*

$$1 - Ch \le \|[\nabla\boldsymbol{F}_T^l]^{-1}\|_{L^\infty(T^1)} \le 1 + Ch, \quad \|[\nabla\boldsymbol{F}_T^l]^{-1} - \mathbf{I}\|_{L^\infty(T^1)} \le Ch, \tag{SM2.13}$$

*where* $C$ *only depends on* $\Gamma$.

*Proof.* The first estimate in (SM2.12) follows from (SM2.7) with $l = 1$, and also implies that

$$\|\nabla^s\boldsymbol{F}^l\|_{L^\infty(T^1)} \le C_s, \quad \text{for } s = 0,1,2, \tag{SM2.14}$$

where $C_0 = C_1 = O(1)$, and $C_2 > 0$ depends on the curvature of $\Gamma$. In particular, this implies that $\|[\nabla\boldsymbol{F}^l]^{-1}\|_{L^\infty(T^1)} = O(1)$, which gives

$$\begin{aligned} \|[\nabla\boldsymbol{F}^l]^{-1} - \mathbf{I}\|_{L^\infty(T^1)} &\le \|[\nabla\boldsymbol{F}^l]^{-1}\|_{L^\infty(T^1)}\|\mathbf{I} - [\nabla\boldsymbol{F}^l]\|_{L^\infty(T^1)} \\ &\le C\|\nabla(\boldsymbol{F}^l - \mathrm{id}_{T^1})\|_{L^\infty(T^1)} \le Ch, \end{aligned} \tag{SM2.15}$$

using the first estimate in (SM2.12). This proves (SM2.13). Then,

$$\begin{aligned} &\|\nabla^s(\boldsymbol{F}_T^m - \boldsymbol{F}_T^l)\|_{L^\infty(T^1)} = \|\nabla^s[(\boldsymbol{\Phi}_T^{lm} - \mathrm{id}_{T^l}) \circ \boldsymbol{F}_T^l]\|_{L^\infty(T^1)} \\ &\quad \le C\sum_{j=1}^{s}\|\nabla^j(\boldsymbol{\Phi}_T^{lm} - \mathrm{id}_{T^l})\|_{L^\infty(T^1)}\|\nabla^{s-j+1}\boldsymbol{F}_T^l\|_{L^\infty(T^1)} \le Ch^{l+1-s}, \end{aligned} \tag{SM2.16}$$

for $0 \le s \le l+1$, where we used the product rule, (SM2.7), (SM2.14), and many inverse estimates. ∎

Corollary SM2.5. *The map* $\boldsymbol{\Phi}^{lm}$ *satisfies the following identities:*

$$\begin{aligned} \left[\boldsymbol{\Phi}^{lm} - \mathrm{id}_{T^l}\right] \circ \boldsymbol{F}^l &= \boldsymbol{F}^m - \boldsymbol{F}^l, \\ \left[\nabla(\boldsymbol{\Phi}^{lm} - \mathrm{id}_{T^l})\right] \circ \boldsymbol{F}^l &= \nabla(\boldsymbol{F}^m - \boldsymbol{F}^l) + O(h^{l+1}), \\ \left[\nabla^2(\boldsymbol{\Phi}^{lm} - \mathrm{id}_{T^l}) \cdot \mathbf{e}_\gamma\right] \circ \boldsymbol{F}^l &= \nabla^2(\boldsymbol{F}^m - \boldsymbol{F}^l) \cdot \mathbf{e}_\gamma + O(h^l), \end{aligned} \tag{SM2.17}$$

*for* $\gamma = 1,2$, *where the constants depend on* $\Gamma \in C^{k+1}$, *and* $l \le m \le k$.

*Proof.* We start by noting that $\boldsymbol{\Phi}^{lm} - \mathrm{id}_{T^l} = (\boldsymbol{F}^m - \boldsymbol{F}^l) \circ (\boldsymbol{F}^l)^{-1}$, and so

$$\begin{aligned} \nabla(\boldsymbol{\Phi}^{lm} - \mathrm{id}_{T^l}) &= ([\nabla(\boldsymbol{F}^m - \boldsymbol{F}^l)][\nabla \boldsymbol{F}^l]^{-1}) \circ (\boldsymbol{F}^l)^{-1}, \\ \nabla^2(\boldsymbol{\Phi}^{lm} - \mathrm{id}_{T^l}) &= ([\nabla^2(\boldsymbol{F}^m - \boldsymbol{F}^l)] : [[\nabla \boldsymbol{F}^l]^{-1} \otimes [\nabla \boldsymbol{F}^l]^{-1}]) \circ (\boldsymbol{F}^l)^{-1} \\ &\quad -(\nabla(\boldsymbol{F}^m - \boldsymbol{F}^l) \left[[\nabla \boldsymbol{F}^l]^{-T}[\nabla^2 \boldsymbol{F}^l][\nabla \boldsymbol{F}^l]^{-1}\right] [\nabla \boldsymbol{F}^l]^{-1}) \circ (\boldsymbol{F}^l)^{-1}, \end{aligned} \tag{SM2.18}$$

and so

$$\begin{aligned} [\nabla(\boldsymbol{\Phi}^{lm} - \mathrm{id}_{T^l})] \circ \boldsymbol{F}^l &= [\nabla(\boldsymbol{F}^m - \boldsymbol{F}^l)][\nabla \boldsymbol{F}^l]^{-1} \\ &= [\nabla(\boldsymbol{F}^m - \boldsymbol{F}^l)] \left\{[\nabla \boldsymbol{F}^l]^{-1} - \mathbf{I}\right\} + \nabla(\boldsymbol{F}^m - \boldsymbol{F}^l) \\ &\leq \nabla(\boldsymbol{F}^m - \boldsymbol{F}^l) + Ch^{l+1}, \end{aligned} \tag{SM2.19}$$

where we used (SM2.12) and (SM2.13). Next, we have

$$\begin{aligned} [\nabla^2(\boldsymbol{\Phi}^{lm} - \mathrm{id}_{T^l}) \cdot \mathbf{e}_\gamma] \circ \boldsymbol{F}^l &= [\nabla \boldsymbol{F}^l]^{-T}[\nabla^2(\boldsymbol{F}^m - \boldsymbol{F}^l) \cdot \mathbf{e}_\gamma][\nabla \boldsymbol{F}^l]^{-1} \\ &\quad -(\nabla(\boldsymbol{F}^m - \boldsymbol{F}^l) \cdot \mathbf{e}_\gamma) \left[[\nabla \boldsymbol{F}^l]^{-T}[\nabla^2 \boldsymbol{F}^l][\nabla \boldsymbol{F}^l]^{-1}\right] [\nabla \boldsymbol{F}^l]^{-1} \\ &\leq \nabla^2(\boldsymbol{F}^m - \boldsymbol{F}^l) \cdot \mathbf{e}_\gamma + Ch^l, \end{aligned} \tag{SM2.20}$$

where we add/subtract the identity matrix and use (SM2.12)–(SM2.14). ∎

### SM2.4. Proof of Proposition 3.3.

*Proof.* W.L.O.G., assume $m > l$. From [SM5, Prop. 4], $\|v\|_{H^s(T^m)} \approx \|\hat{v}\|_{H^s(T^l)}$ for $s \geq 0$. More specifically, $\|\nabla v\|_{L^2(\mathcal{T}_h^m)} \approx \|\nabla \hat{v}\|_{L^2(\mathcal{T}_h^l)}$ and

$$\|\nabla^2 v\|_{L^2(\mathcal{T}_h^m)} \leq C \left(\|\nabla^2 \hat{v}\|_{L^2(\mathcal{T}_h^l)} + h^{l-1}\|\nabla \hat{v}\|_{L^2(\mathcal{T}_h^l)}\right).$$

Applying a change of variables to the jump term in (2.10) gives

$$\| [\![\boldsymbol{n} \cdot \nabla v]\!] \|_{L^2(\mathcal{E}_h^m)} \leq Ch^l\|\nabla \hat{v}\|_{L^2(\mathcal{E}_h^l)} + \| [\![\hat{\boldsymbol{n}} \cdot \nabla \hat{v}]\!] \|_{L^2(\mathcal{E}_h^l)}, \tag{SM2.21}$$

where we emphasize that we cannot put a jump in the first term on the right-hand-side because different Jacobians appear on either side of the edge. Next, we have the following scaling estimate (see (2.8))

$$\|\nabla \hat{v}\|^2_{L^2(\partial T^l)} \leq C_0 \left(h^{-1}\|\nabla \hat{v}\|^2_{L^2(T^l)} + h\|\nabla^2 \hat{v}\|^2_{L^2(T^l)}\right), \tag{SM2.22}$$

which leads to

$$h^{-1/2}\| [\![\boldsymbol{n} \cdot \nabla v]\!] \|_{L^2(\mathcal{E}_h^m)} \leq C_1 h^{l-1}\|\nabla \hat{v}\|_{L^2(\mathcal{T}_h^l)} + C_1 h^l\|\nabla^2 \hat{v}\|_{L^2(\mathcal{T}_h^l)} + h^{-1/2}\| [\![\hat{\boldsymbol{n}} \cdot \nabla \hat{v}]\!] \|_{L^2(\mathcal{E}_h^l)}, \tag{SM2.23}$$

and implies $\|v\|_{2,h,m} \leq C_2(\|\hat{v}\|_{2,h,l} + h^{l-1}\|\nabla \hat{v}\|_{L^2(\Omega^l)})$, giving the upper bound in (3.5) and (3.6). Combining with the Poincaré inequality in (2.14), shows the upper bound in (3.6); the lower bound follows similarly.

For $\|v\|_{0,h,m}$, the argument is simpler because there are no jump terms. ∎

## SM3. Mesh-dependent Approximation Results for Curved Lagrange Finite Elements.

**SM3.1. Scaling Results.**

LEMMA SM3.1. *Assume $1 \leq m \leq k$ (or $m = \infty$). There is a constant $C > 0$, independent of $h$ and $m$, such that*

$$\|v\|_{L^q(\partial T^m)} \leq C h^{1/q-2/p} \|v\|_{L^p(T^m)}, \quad \text{for any } 1 \leq q, p \leq \infty, \tag{SM3.1}$$

*for all $\hat{v} := v \circ \boldsymbol{F}_T^m \in \mathcal{P}_r(T^1)$, where $r \geq 0$.*

COROLLARY SM3.2. *Assume $1 \leq m \leq k$ (or $m = \infty$). There is a constant $C > 0$, independent of $h$ and $m$, such that*

$$\|\nabla v\|_{L^q(\partial T^m)} \leq C h^{1/q-2/p} \|\nabla v\|_{L^p(T^m)}, \ \text{for any } 1 \leq q, p \leq \infty, \tag{SM3.2}$$

*for all $\hat{v} := v \circ \boldsymbol{F}_T^m \in \mathcal{P}_{r+1}(T^1)$, where $r \geq 0$.*

The following mesh-dependent results essentially come from [SM1] (when $m = 1$).

LEMMA SM3.3. *Assume $1 \leq m \leq k$ (or $m = \infty$). There is a constant $C > 0$, independent of $h$ and $m$, such that*

$$\|v\|_{0,h} \leq C \|v\|_{L^2(\Omega^m)}, \quad \text{for all } v \in W_h^m, \tag{SM3.3}$$

*where $\|\cdot\|_{0,h}$ is given in (2.12).*

*Proof.* Combining Proposition 2.1 with an inverse inequality gives the assertion. ∎

LEMMA SM3.4. *Assume $1 \leq m \leq k$ (or $m = \infty$). There is a constant $C > 0$, independent of $h$ and $m$, such that*

$$\|v\|_{2,h} \leq C h^{-1} \|v\|_{H^1(\Omega^m)}, \quad \text{for all } v \in W_h^m. \tag{SM3.4}$$

**SM3.2. Approximation Results.** The following approximation results follow from [SM1] when $m = 1$.

LEMMA SM3.5. *Suppose $v \in W^{t,p}(\Omega^m)$, for $p > 1$ and $t \geq 2$ is an integer. Then,*

$$\|\nabla^s (v - \mathcal{I}_h^m v)\|_{L^q(\mathcal{E}_h^m)} \leq C h^{l-s+1/q-2/p+2\min(0,1/p-1/q)} \|v\|_{W^{l,p}(\Omega^m)}, \tag{SM3.5}$$

*where $s = 0, 1$, $1 \leq l \leq \min(r+2, t)$, for all $h$, and $C > 0$ is an independent constant, and $1 \leq q \leq \infty$ is such that $W^{l,p}(\widehat{T}) \hookrightarrow W^{s,q}(\partial \widehat{T})$.*

LEMMA SM3.6. *Assume the hypothesis of Lemma SM3.5. Then,*

$$\begin{aligned} \|\nabla^s (v - \mathcal{I}_h^m v)\|_{L^q(\Omega^m)} &\leq C h^{l-s+2/q-2/p+2\min(0,1/p-1/q)} \|v\|_{W^{l,p}(\Omega^m)}, \\ \|v - \mathcal{I}_h^m v\|_{L^2(\Omega^m)} \leq \|v - \mathcal{I}_h^m v\|_{0,h} &\leq C h^l \|v\|_{H^l(\Omega^m)}, \ \text{for } v \in H^l(\Omega^m) \cap W^{t,p}(\Omega^m), \end{aligned} \tag{SM3.6}$$

*where $s = 0, 1$, $1 \leq l \leq \min(r+2, t)$, for all $h$, $C > 0$ is an independent constant, and $1 \leq q \leq \infty$ is such that $W^{l,p}(\widehat{T}) \hookrightarrow W^{s,q}(\widehat{T})$.*

LEMMA SM3.7. *Assume the hypothesis of Lemma SM3.5. Then,*

$$\begin{aligned} \left( \sum_{T^m \in \mathcal{T}_h^m} |v - \mathcal{I}_h^m v|^q_{W^{2,q}(T^m)} \right)^{1/q} &\leq C h^{l-2+2/q-2/p+2\min(0,1/p-1/q)} \|v\|_{W^{l,p}(\Omega^m)}, \\ \|v - \mathcal{I}_h^m v\|_{2,h} &\leq C h^{l-1-2/p} \|v\|_{W^{l,p}(\Omega^m)}, \end{aligned} \tag{SM3.7}$$

*where* $2 \leq l \leq \min(r+2,t)$*, for all* $h$*,* $C > 0$ *is an independent constant, and* $1 \leq q \leq \infty$ *is such that* $W^{l,p}(\widehat{T}) \hookrightarrow W^{2,q}(\widehat{T})$*.*

*Proof.* The first inequality is standard. The second follows by recalling the definition (2.10) and combining the first inequality and (SM3.5) with $q = 2$. ∎

**SM4. Approximation Results for Curved HHJ Finite Elements.** We make note of some standard transformation rules for covariant and contravariant quantities, since they are critical for analyzing the geometric error when comparing similar quantities on different domains, e.g. $\Omega^m$ and $\Omega^l$ with $m \neq l$.

We use a "hat" notation to indicate a function defined on $T^1$. Recall the following transformation rules for covariant (contravariant) vectors and tensors:

$$\begin{aligned} &\text{(covariant)} \quad \boldsymbol{v} \circ \boldsymbol{F}_T^m(\hat{\boldsymbol{u}}) = (\boldsymbol{B}_T^m)^{-T}\hat{\boldsymbol{v}}, \\ &\text{(contravariant)} \quad \boldsymbol{v} \circ \boldsymbol{F}_T^m(\hat{\boldsymbol{u}}) = \boldsymbol{B}_T^m\hat{\boldsymbol{v}}, \\ &\text{(covariant)} \quad \boldsymbol{w} \circ \boldsymbol{F}_T^m(\hat{\boldsymbol{u}}) = (\boldsymbol{B}_T^m)^{-T}\hat{\boldsymbol{w}}(\boldsymbol{B}_T^m)^{-1}, \\ &\text{(contravariant)} \quad \boldsymbol{w} \circ \boldsymbol{F}_T^m(\hat{\boldsymbol{u}}) = \boldsymbol{B}_T^m\hat{\boldsymbol{w}}(\boldsymbol{B}_T^m)^{T}, \end{aligned} \tag{SM4.1}$$

where $\boldsymbol{B}_T^m := \nabla \boldsymbol{F}_T^m$.

We also note the following transformation rules for normal and tangent vectors on $\partial T$:

$$\boldsymbol{n} \circ \boldsymbol{F}_T^m = \frac{(\boldsymbol{B}_T^m)^{-T}\hat{\boldsymbol{n}}}{|(\boldsymbol{B}_T^m)^{-T}\hat{\boldsymbol{n}}|}, \qquad \boldsymbol{t} \circ \boldsymbol{F}_T^m = \frac{\boldsymbol{B}_T^m\hat{\boldsymbol{t}}}{|\boldsymbol{B}_T^m\hat{\boldsymbol{t}}|}. \tag{SM4.2}$$

**SM4.1. The Reference HHJ Element.** Recall (4.1) and let

$$V_h^1 \equiv V_h^1(T^1) := \mathcal{P}_r(T^1;\mathbb{S}) \subset \mathcal{M}_{\mathrm{nn}}^1(T^1),$$

be a conforming finite element space on the element $T^1 \in \mathcal{T}_h^1$ with nodal Degrees-of-Freedom (DoFs) given by

$$\begin{aligned} &\bullet\ |E^1| \int_{E^1} \hat{\boldsymbol{n}}^T \hat{\boldsymbol{\varphi}} \hat{\boldsymbol{n}} \hat{q}\, ds, \ \forall \hat{q} \in \mathcal{P}_r(E^1), \ \forall E^1 \in \partial T^1, \\ &\bullet\ \int_{T^1} \hat{\boldsymbol{\varphi}} : \hat{\boldsymbol{\eta}}\, d\mathrm{S}, \ \forall \hat{\boldsymbol{\eta}} \in \mathcal{P}_{r-1}(T^1;\mathbb{S}), \end{aligned} \tag{SM4.3}$$

i.e. $\hat{\boldsymbol{\varphi}} \in V_h^1$ is uniquely defined by (SM4.3) [SM6].

**SM4.2. Matrix Piola Transform.** We now recall Definition 4.2 of the matrix Piola transform, and verify a key elementary property, which shows that it preserves normal-normal continuity. Given an orientation-preserving diffeomorphism $\boldsymbol{F} : \widehat{\mathcal{D}} \to \mathcal{D}$, and a tensor field $\boldsymbol{\varphi} : \mathcal{D} \to \mathbb{R}^2$, we define $\hat{\boldsymbol{\varphi}} : \widehat{\mathcal{D}} \to \mathbb{R}^2$ by

$$\hat{\boldsymbol{\varphi}}(\hat{\mathbf{x}}) = (\det \boldsymbol{B})^2 \boldsymbol{B}^{-1} \boldsymbol{\varphi}(\mathbf{x}) \boldsymbol{B}^{-T},$$

where $\mathbf{x} = \boldsymbol{F}(\hat{\mathbf{x}})$, and $\boldsymbol{B} = \boldsymbol{B}(\hat{\mathbf{x}}) = \nabla \boldsymbol{F}(\hat{\mathbf{x}})$. Also, denote by $\boldsymbol{t}, \boldsymbol{n} : \partial\mathcal{D} \to \mathbb{R}^2$ the positively-oriented unit tangent vector and the outward unit normal vector, and similarly for $\hat{\boldsymbol{t}}, \hat{\boldsymbol{n}}$ on $\partial\widehat{\mathcal{D}}$. Then the normal-normal component of $\varphi$ transforms as follows:

$$(\hat{\boldsymbol{n}}^T \hat{\boldsymbol{\varphi}} \hat{\boldsymbol{n}}) |\boldsymbol{B}\hat{\boldsymbol{t}}|^{-2} = (\boldsymbol{n}^T \boldsymbol{\varphi} \boldsymbol{n}) \circ \boldsymbol{F}. \tag{SM4.4}$$

To see this, note that $\boldsymbol{t} = |\boldsymbol{B}\hat{\boldsymbol{t}}|^{-1}\boldsymbol{B}\hat{\boldsymbol{t}}$ and $\boldsymbol{n} = |\boldsymbol{B}^{-T}\hat{\boldsymbol{n}}|^{-1}\boldsymbol{B}^{-T}\hat{\boldsymbol{n}} = (\det \boldsymbol{B})|\boldsymbol{B}\hat{\boldsymbol{t}}|^{-1}\boldsymbol{B}^{-T}\hat{\boldsymbol{n}}$, where we have used the elementary identity $(\det \boldsymbol{B})|\boldsymbol{B}^{-T}\hat{\boldsymbol{n}}| = |\boldsymbol{B}\hat{\boldsymbol{t}}|$, whenever $\boldsymbol{B}$ is a $2 \times 2$ matrix with positive determinant and $\hat{\boldsymbol{t}}$, $\hat{\boldsymbol{n}}$ are orthonormal. Thus $\hat{\boldsymbol{n}} = (\det \boldsymbol{B})^{-1}|\boldsymbol{B}\hat{\boldsymbol{t}}|\boldsymbol{B}^T\boldsymbol{n}$. Substituting this expression and the definition of $\hat{\boldsymbol{\varphi}}$ into the left-hand size of (SM4.4) gives the result.

Note that the term $\boldsymbol{B}\hat{\boldsymbol{t}}$ in (SM4.4) is *continuous* across inter-element boundaries. Indeed, for $\varphi^{\mathrm{nn}}$, we have

$$\varphi^{\mathrm{nn}} \circ \boldsymbol{F}_T^m \equiv (\boldsymbol{n}^T\boldsymbol{\varphi}\boldsymbol{n}) \circ \boldsymbol{F}_T^m = |\boldsymbol{B}_T^m\hat{\boldsymbol{t}}|^{-2}\hat{\varphi}^{\mathrm{nn}}. \tag{SM4.5}$$

Hence, one can map basis functions on the reference element to basis functions on the physical element using (4.2) and maintain normal-normal continuity. Furthermore, if $\boldsymbol{F}$ is a general affine map ($m = 1$), with $E = \boldsymbol{F}(E^1)$, then $|\boldsymbol{B}\hat{\boldsymbol{t}}| = |E|/|E^1|$, so (SM4.4) implies that

$$|E|\int_E (\boldsymbol{n}^T\boldsymbol{\varphi}\boldsymbol{n})q\,ds = |E^1|\int_{E^1}(\hat{\boldsymbol{n}}^T\hat{\boldsymbol{\varphi}}\hat{\boldsymbol{n}})\hat{q}\,ds, \quad \forall \hat{q} \in \mathcal{P}_r(E^1), \text{ and all edges } E^1 \text{ in } \partial T^1, \tag{SM4.6}$$

i.e. the edge DoFs are scaled when mapped.

We close with a norm equivalence implied by Lemma SM3.3:

$$\|\boldsymbol{\varphi}\|_{0,h}^2 \le C_0 \sum_{\alpha,\beta=1}^{2} \|\varphi^{\alpha\beta}\|_{0,h}^2 \le CC_0\|\boldsymbol{\varphi}\|_{L^2(\Omega^m)}^2, \quad \forall \boldsymbol{\varphi} \in V_h^m, \tag{SM4.7}$$

so $\|\boldsymbol{\varphi}\|_{0,h} \approx \|\boldsymbol{\varphi}\|_{L^2(\Omega)}$ for all $\boldsymbol{\varphi} \in V_h^m$. By the same arguments in the proof of Proposition 3.3, we have that

$$\|\boldsymbol{\varphi}\|_{0,h,m} \approx \|\hat{\boldsymbol{\varphi}}\|_{0,h,l}, \text{ for all } \boldsymbol{\varphi} \in H_h^0(\Omega^m;\mathbb{S}), \tag{SM4.8}$$

using the Piola transform involving $\boldsymbol{\Phi}$ taken from Proposition 3.3.

**SM4.3. Approximation Results of the HHJ Interpolation Operator.** The operator $\Pi_h^m$ enjoys the following approximation properties [SM4].

Lemma SM4.1. *Suppose $\boldsymbol{\varphi} \in W^{t,p}(\Omega^m;\mathbb{S})$, for $p > 1$ and $t \ge 1$ is an integer. Then,*

$$\|\boldsymbol{\varphi} - \Pi_h^m\boldsymbol{\varphi}\|_{L^q(\mathcal{E}_h^m)} \le Ch^{l+1/q-2/p+2\min(0,1/p-1/q)}\|\boldsymbol{\varphi}\|_{W^{l,p}(\Omega^m)}, \tag{SM4.9}$$

*where $1 \le l \le \min(r+1,t)$, for all $h$, and $C > 0$ is an independent constant, and $1 \le q \le \infty$ is such that $W^{l,p}(\widehat{T}) \hookrightarrow L^q(\partial\widehat{T})$.*

The following is a modification of [SM4, Lem. 4].

Lemma SM4.2. *For $2 \ge p > 1$ and $t \ge 1$ is an integer, there holds*

$$\begin{aligned} \|\Pi_h^m\boldsymbol{\varphi}\|_{\mathcal{M}_{\mathrm{nn}}^m(\Omega^m)} &\le C\|\boldsymbol{\varphi}\|_{\mathcal{M}_{\mathrm{nn}}^m(\Omega^m)}, \quad \text{for all } \boldsymbol{\varphi} \in \mathcal{M}_{\mathrm{nn}}^m(\Omega^m), \\ \|\boldsymbol{\varphi} - \Pi_h^m\boldsymbol{\varphi}\|_{L^q(\Omega^m)} &\le Ch^{l+2(1/q-1/p)+2\min(0,1/p-1/q)}\|\boldsymbol{\varphi}\|_{W^{l,p}(\Omega^m)}, \\ \|\boldsymbol{\varphi} - \Pi_h^m\boldsymbol{\varphi}\|_{L^2(\Omega^m)} &\le \|\boldsymbol{\varphi} - \Pi_h^m\boldsymbol{\varphi}\|_{0,h} \le Ch^{l+1-2/p}\|\boldsymbol{\varphi}\|_{W^{l,p}(\Omega^m)}, \end{aligned} \tag{SM4.10}$$

*for all $\boldsymbol{\varphi} \in \mathcal{M}_{\mathrm{nn}}^m(\Omega^m) \cap W^{t,p}(\Omega^m)$, where $\|\boldsymbol{\varphi}\|_{\mathcal{M}_{\mathrm{nn}}^m(\Omega^m)}^p := \|\boldsymbol{\varphi}\|_{L^p(\Omega^m)}^p + \sum_{T^m}\|\nabla\boldsymbol{\varphi}\|_{L^p(T^m)}^p$, $1 \le l \le \min(r+1,t)$, for all $h$, $C > 0$ is an independent constant, and $1 \le q \le \infty$ is such that $W^{l,p}(\widehat{T}) \hookrightarrow L^q(\widehat{T})$.*

We have the following scaling result.

LEMMA SM4.3. *There is a constant $C > 0$, independent of $h$ and $m$, such that*

$$\|\boldsymbol{n}^T \boldsymbol{\varphi} \boldsymbol{n}\|_{L^q(\partial T^m)} \leq \|\boldsymbol{\varphi}\|_{L^q(\partial T^m)} \leq C h^{1/q-2/p} \|\boldsymbol{\varphi}\|_{L^p(T^m)}, \quad \text{for any } 1 \leq q, p \leq \infty, \tag{SM4.11}$$

*for all* $\hat{\boldsymbol{\varphi}} := (\det \boldsymbol{B}_T^m)^2 (\boldsymbol{B}_T^m)^{-1} (\boldsymbol{\varphi} \circ \boldsymbol{F}_T^m)(\boldsymbol{B}_T^m)^{-T} \in \mathcal{P}_r(T^1; \mathbb{S})$, *where* $r \geq 0$.

**SM5. Discrete Inf-Sup Condition.** We recall [SM2, Lem. 5.1].

LEMMA SM5.1. *Assume the domain $\Omega$ is piecewise linear, i.e. $m = 1$. Then,*

$$\sup_{\boldsymbol{\varphi} \in V_h^1} \frac{|b_h^1(\boldsymbol{\varphi}, v)|}{\|\boldsymbol{\varphi}\|_{0,h,1}} \geq C_0 \|v\|_{2,h,1}, \quad \forall v \in W_h^1, \ \forall h > 0, \tag{SM5.1}$$

*holds for any degree $r \geq 0$, where $C_0 > 0$ is independent of $h$.*

**SM6. Proof of Theorem 5.2.** In lieu of Remark 4.7, we let $|||\cdot|||_h$ denote any norm on $W_h$ for which the inf-sup condition holds.

**Step 1.** First, form the usual "error equations":

$$a(\boldsymbol{\sigma} - \boldsymbol{\sigma}_h, \boldsymbol{\varphi}_h) + b_h(\boldsymbol{\varphi}_h, w - w_h) + b_h(\boldsymbol{\sigma} - \boldsymbol{\sigma}_h, v_h) = 0, \tag{SM6.1}$$

for all $(v_h, \boldsymbol{\varphi}_h) \in W_h \times V_h$. By the standard theory of mixed methods, one obtains the following abstract convergence result as a special case of [SM3, Thm. 5.2.1]:

$$\begin{aligned} \|\boldsymbol{\sigma}_h - \boldsymbol{\varphi}_h\|_{0,h} \leq{}& \frac{1}{\alpha_0} \sup_{\boldsymbol{\omega}_h \in V_h} \frac{|a(\boldsymbol{\sigma} - \boldsymbol{\varphi}_h, \boldsymbol{\omega}_h) + b_h(\boldsymbol{\omega}_h, w - v_h)|}{\|\boldsymbol{\omega}_h\|_{0,h}} \\ &+ \frac{1}{\beta_0} \left(\frac{A_0}{\alpha_0}\right)^{1/2} \sup_{z_h \in W_h} \frac{|b_h(\boldsymbol{\sigma} - \boldsymbol{\varphi}_h, z_h)|}{|||z_h|||_h}, \end{aligned} \tag{SM6.2}$$

$$\begin{aligned} |||w_h - v_h|||_h \leq{}& \frac{C}{\beta_0} \left(1 + \frac{A_0^{1/2}}{\alpha_0^{1/2}}\right) \sup_{\boldsymbol{\omega}_h \in V_h} \frac{|a(\boldsymbol{\sigma} - \boldsymbol{\varphi}_h, \boldsymbol{\omega}_h) + b_h(\boldsymbol{\omega}_h, w - v_h)|}{\|\boldsymbol{\omega}_h\|_{0,h}} \\ &+ \frac{C_{\mathrm{P}}^2 A_0}{\beta_0^2} \sup_{z_h \in W_h} \frac{|b_h(\boldsymbol{\sigma} - \boldsymbol{\varphi}_h, z_h)|}{|||z_h|||_h}, \end{aligned} \tag{SM6.3}$$

for all $v_h \in W_h$, $\boldsymbol{\varphi}_h \in V_h$. Next, set $v_h = \mathcal{I}_h w$, $\boldsymbol{\varphi}_h = \Pi_h \boldsymbol{\sigma}$.

**Step 2.** Let $l_1 := \min(r+1, t-2)$ and $l_2 := \min(r+2, t)$. If $|||\cdot|||_h = \|\cdot\|_{2,h}$, (4.21), (4.31) and the interpolation estimates (SM3.7), (SM4.10) imply

$$\begin{aligned} \|\boldsymbol{\sigma}_h - \Pi_h \boldsymbol{\sigma}\|_{0,h} + \|w_h - \mathcal{I}_h w\|_{2,h} \leq{}& C\|\boldsymbol{\sigma} - \Pi_h \boldsymbol{\sigma}\|_{0,h} \\ &+ C\|\nabla(w - \mathcal{I}_h w)\|_{L^2(\Omega_S)} + Ch\|\nabla^2(w - \mathcal{I}_h w)\|_{L^2(\mathcal{T}_{\partial,h})} \\ \leq{}& C\left(h^{l_1+1-2/p}\|\boldsymbol{\sigma}\|_{W^{l_1,p}(\Omega)} + h^{l_2-2/p}\|w\|_{W^{l_2,p}(\Omega)}\right), \end{aligned} \tag{SM6.4}$$

where $C > 0$ is an independent constant.

Therefore, by the triangle inequality,

$$\|\boldsymbol{\sigma} - \boldsymbol{\sigma}_h\|_{0,h} \leq C\left(h^{l_1+1-2/p}\|\boldsymbol{\sigma}\|_{W^{l_1,p}(\Omega)} + h^{l_2-2/p}\|w\|_{W^{l_2,p}(\Omega)}\right), \tag{SM6.5}$$

$$\begin{aligned} \|w - w_h\|_{2,h} \leq{}& C\left(h^{l_1+1-2/p}\|\boldsymbol{\sigma}\|_{W^{l_1,p}(\Omega)}\right) \\ &+ C\min\left\{h^{l_2-1-2/p}\|w\|_{W^{l_2,p}(\Omega)}, \|w\|_{H^2(\Omega)}\right\}, \end{aligned} \tag{SM6.6}$$

for some independent constant $C > 0$.

**Step 3.** If $|||\cdot|||_h = |\cdot|_{H^1(\Omega)}$, (4.21), (4.31) and the interpolation estimates (SM3.7), (SM4.10) imply

$$\begin{aligned}\|\boldsymbol{\sigma}_h - \Pi_h\boldsymbol{\sigma}\|_{0,h} + \|\nabla(w_h - \mathcal{I}_h w)\|_{L^2(\Omega)} &\leq C\|\boldsymbol{\sigma} - \Pi_h\boldsymbol{\sigma}\|_{0,h} \\ &+ C\left(\|\nabla(w - \mathcal{I}_h w)\|_{L^2(\Omega_S)} + h\|\nabla^2(w - \mathcal{I}_h w)\|_{L^2(\mathcal{T}_{\partial,h})}\right) \\ &\leq Ch^{l_1+1-2/p}\|\boldsymbol{\sigma}\|_{W^{l_1,p}(\Omega)} + Ch^{l_2-2/p}\|w\|_{W^{l_2,p}(\Omega)},\end{aligned} \tag{SM6.7}$$

Therefore, by the triangle inequality,

$$\|\boldsymbol{\sigma} - \boldsymbol{\sigma}_h\|_{0,h} + \|\nabla(w - w_h)\|_{L^2(\Omega)} \leq C\left(h^{l_1+1-2/p}\|\boldsymbol{\sigma}\|_{W^{l_1,p}(\Omega)} + h^{l_2-2/p}\|w\|_{W^{l_2,p}(\Omega)}\right), \tag{SM6.8}$$

for some independent constant $C > 0$.

**Step 4.** We use a duality argument to get a better estimate for $\|\nabla(w-w_h)\|_{L^2(\Omega)}$, in the low regularity case and when $r = 0$. Let $d \in H^{-1}(\Omega)$, and let $\boldsymbol{\tau} \in V$, $\rho \in W$ solve (2.17) with $f$ replaced by $d$, i.e.

$$a(\boldsymbol{\varphi}, \boldsymbol{\tau}) + b_h(\boldsymbol{\tau}, v) + b_h(\boldsymbol{\varphi}, \rho) = -\langle d, v\rangle, \quad \forall(\boldsymbol{\varphi}, v) \in V \times W. \tag{SM6.9}$$

Then, $\|\boldsymbol{\tau}\|_{W^{1,p}(\Omega)} + \|\rho\|_{W^{3,p}(\Omega)} \leq C\|d\|_{H^{-1}(\Omega)}$. Next, set $\boldsymbol{\varphi} = \boldsymbol{\sigma} - \boldsymbol{\sigma}_h$, $v = w - w_h$:

$$-\langle d, w - w_h\rangle = a(\boldsymbol{\sigma} - \boldsymbol{\sigma}_h, \boldsymbol{\tau}) + b_h(\boldsymbol{\tau}, w - w_h) + b_h(\boldsymbol{\sigma} - \boldsymbol{\sigma}_h, \rho). \tag{SM6.10}$$

Next, combine with (SM6.1):

$$\begin{aligned}-\langle d, w - w_h\rangle = a(\boldsymbol{\sigma} - \boldsymbol{\sigma}_h, \boldsymbol{\tau} - \boldsymbol{\varphi}_h) + b_h(\boldsymbol{\tau} - \boldsymbol{\varphi}_h, w - w_h) \\ + b_h(\boldsymbol{\sigma} - \boldsymbol{\sigma}_h, \rho - v_h), \quad \forall(\boldsymbol{\varphi}_h, v_h) \in V_h \times W_h.\end{aligned} \tag{SM6.11}$$

Now set $v_h = \mathcal{I}_h\rho$, $\boldsymbol{\varphi}_h = \Pi_h\boldsymbol{\tau}$:

$$\begin{aligned}|\langle d, w - w_h\rangle| \leq |a(\boldsymbol{\sigma} - \boldsymbol{\sigma}_h, \boldsymbol{\tau} - \Pi_h\boldsymbol{\tau})| + |b_h(\boldsymbol{\tau} - \Pi_h\boldsymbol{\tau}, w - w_h)| \\ + |b_h(\boldsymbol{\sigma} - \boldsymbol{\sigma}_h, \rho - \mathcal{I}_h\rho)|.\end{aligned} \tag{SM6.12}$$

Let us estimate the terms involving $b_h(\cdot,\cdot)$. First, adding and subtracting $\mathcal{I}_h w$:

$$\begin{aligned}|b_h(\boldsymbol{\tau} - \Pi_h\boldsymbol{\tau}, w - w_h)| &\leq |b_h(\boldsymbol{\tau} - \Pi_h\boldsymbol{\tau}, w - \mathcal{I}_h w)| + |b_h(\boldsymbol{\tau} - \Pi_h\boldsymbol{\tau}, \mathcal{I}_h w - w_h)| \\ &\leq |b_h(\boldsymbol{\tau}, w - \mathcal{I}_h w)| \\ &\quad + |b_h(\Pi_h\boldsymbol{\tau}, w - \mathcal{I}_h w)| + |b_h(\boldsymbol{\tau} - \Pi_h\boldsymbol{\tau}, \mathcal{I}_h w - w_h)| \\ &\leq |\langle d, w - \mathcal{I}_h w\rangle| \\ &\quad + C\|\Pi_h\boldsymbol{\tau}\|_{L^2(\Omega_S)}\left(\|\nabla(w - \mathcal{I}_h w)\|_{L^2(\Omega_S)} + h\|\nabla^2(w - \mathcal{I}_h w)\|_{L^2(\mathcal{T}_{\partial,h})}\right), \\ &\quad + C\|\boldsymbol{\tau} - \Pi_h\boldsymbol{\tau}\|_{H_h^0(\Omega_S)}\|\nabla(\mathcal{I}_h w - w_h)\|_{L^2(\Omega_S)},\end{aligned} \tag{SM6.13}$$

where we used (SM6.9) (for $\boldsymbol{\tau}$) and (4.21). Interpolation estimates, for $r = 0$ and minimal regularity, and (SM6.7) give

$$\begin{aligned}|b_h(\boldsymbol{\tau} - \Pi_h\boldsymbol{\tau}, w - w_h)| &\leq C\|d\|_{H^{-1}(\Omega)}\left(\|\nabla(w - \mathcal{I}_h w)\|_{L^2(\Omega)} + h\|\nabla^2(w - \mathcal{I}_h w)\|_{L^2(\mathcal{T}_{\partial,h})}\right) \\ &\quad + C\|\boldsymbol{\tau} - \Pi_h\boldsymbol{\tau}\|_{H_h^0(\Omega_S)}\|\nabla(\mathcal{I}_h w - w_h)\|_{L^2(\Omega_S)} \\ &\leq C\left[h + \left(h^{2-2/p}\right)^2\right]\|d\|_{H^{-1}(\Omega)}\|f\|_{H^{-1}(\Omega)}.\end{aligned} \tag{SM6.14}$$

For the next term, we use (2.17) (for $\boldsymbol{\sigma}$) and (4.21):

$$\begin{aligned}|b_h(\boldsymbol{\sigma}-\boldsymbol{\sigma}_h,\rho-\mathcal{I}_h\rho)| &\leq |b_h(\boldsymbol{\sigma},\rho-\mathcal{I}_h\rho)|+|b_h(\boldsymbol{\sigma}_h,\rho-\mathcal{I}_h\rho)| \\ &\leq |\langle f,\rho-\mathcal{I}_h\rho\rangle| \\ &\quad +C\|\boldsymbol{\sigma}_h\|_{L^2(\Omega_S)}\left(\|\nabla(\rho-\mathcal{I}_h\rho)\|_{L^2(\Omega_S)}+h\|\nabla^2(\rho-\mathcal{I}_h\rho)\|_{L^2(\mathcal{T}_{\partial,h})}\right),\end{aligned} \tag{SM6.15}$$

Again, interpolation estimates, for $r=0$ and minimal regularity give

$$\begin{aligned}|b_h(\boldsymbol{\sigma}-\boldsymbol{\sigma}_h,\rho-\mathcal{I}_h\rho)| &\leq C\|f\|_{H^{-1}(\Omega)}\Big[\|\nabla(\rho-\mathcal{I}_h\rho)\|_{L^2(\Omega)} \\ &\qquad +h\|\nabla^2(\rho-\mathcal{I}_h\rho)\|_{L^2(\mathcal{T}_{\partial,h})}\Big] \\ &\leq Ch\|f\|_{H^{-1}(\Omega)}\|d\|_{H^{-1}(\Omega)}.\end{aligned} \tag{SM6.16}$$

**Step 5.** Lastly, for $r=0$ and minimal regularity, we have

$$\begin{aligned}|a(\boldsymbol{\sigma}-\boldsymbol{\sigma}_h,\boldsymbol{\tau}-\Pi_h\boldsymbol{\tau})| &\leq C\|\boldsymbol{\sigma}-\boldsymbol{\sigma}_h\|_{L^2(\Omega)}\|\boldsymbol{\tau}-\Pi_h\boldsymbol{\tau}\|_{L^2(\Omega)} \\ &\leq Ch^{2-2/p}\left(h^{2-2/p}\right)\|d\|_{H^{-1}(\Omega)}\|f\|_{H^{-1}(\Omega)},\end{aligned} \tag{SM6.17}$$

where we used (SM6.5). Therefore,

$$\begin{aligned}\|\nabla(w-w_h)\|_{L^2(\Omega)} &\leq C\sup_{d\in H^{-1}(\Omega)}\frac{\langle d,w-w_h\rangle}{\|d\|_{H^{-1}(\Omega)}} \\ &\leq C\max\left(h,h^{4-4/p}\right)\|f\|_{H^{-1}(\Omega)}.\end{aligned} \tag{SM6.18}$$

## REFERENCES


[SM1] I. Babuška, J. Osborn, and J. Pitkäranta, *Analysis of mixed methods using mesh dependent norms*, Mathematics of Computation, 35 (1980), pp. 1039–1062, http://www.jstor.org/stable/2006374.

[SM2] H. Blum and R. Rannacher, *On mixed finite element methods in plate bending analysis. part 1: The first Herrmann scheme*, Computational Mechanics, 6 (1990), pp. 221–236, https://doi.org/10.1007/BF00350239, https://doi.org/10.1007/BF00350239.

[SM3] D. Boffi, F. Brezzi, and M. Fortin, *Mixed Finite Element Methods and Applications*, vol. 44 of Springer Series in Computational Mathematics, Springer-Verlag, New York, NY, 2013.

[SM4] F. Brezzi and P. A. Raviart, *Mixed finite element methods for 4th order elliptic equations*, in Topics In Numerical Analysis III: Proceedings of the Royal Irish Academy Conference on Numerical Analysis, J. J. H. Miller, ed., Academic Press, 1976, pp. 33–56.

[SM5] M. Lenoir, *Optimal isoparametric finite elements and error estimates for domains involving curved boundaries*, SIAM Journal of Numerical Analysis, 23 (1986), pp. 562–580.

[SM6] L. Li, *Regge Finite Elements with Applications in Solid Mechanics and Relativity*, phd, University of Minnesota, June 2018.
